# Supplementary material for: An Integrated Design Pipeline for Tactile Sensing Robotic Manipulators
Source: arXiv:2204.07149 source file (2022-04-14)
Supplement: Supplementary file 1 [file appendix.tex]

\section*{APPENDIX}

Appendixes should appear before the acknowledgment.
